# Supplementary material for: Instantons and the path to intermittency in turbulent flows
Source: arXiv:2106.08790 ancillary file (2022-06-24)
Supplement: Supplementary file 1 [file SuppMaterial_incl_figures.pdf]

# Instantons and the path to intermittency in turbulent flows

A. Fuchs[1], C. Herbert[2], J. Rolland[3], M. Wächter[1], F. Bouchet[2], J. Peinke[1]
[1] *Institute of Physics and ForWind, University of Oldenburg, Küpkersweg 70, 26129 Oldenburg, Germany*
[2] *Univ. Lyon, Ens de Lyon, Univ Claude Bernard, CNRS, Laboratoire de Physique, F-69364 Lyon, France and*
[3] *Univ. Lille, ONERA, Arts et métiers institute of technology, Centrale Lille, CNRS UMR 9014 -LMFL, Laboratoire de mécanique des Fluides de Lille Kampé de Fériet, 59000 Lille, France*
(Dated: June 14, 2021)

*Appendix A: Kramers-Moyal coefficients.*— The two functions $D^{(1,2)}$ defining the Fokker-Planck equation are called drift and diffusion coefficients, respectively, and are defined by the two first conditional moments ($k = 1, 2$, $s' < s$ and $\Delta s = s - s'$)

$$M^{(k)}\left(u_s, s, \Delta s\right) = \int_{-\infty}^{\infty} \left(u_{s'} - u_s\right)^k p\left(u_{s'}|u_s\right) du_{s'}, \quad (1)$$

known as Kramers-Moyal coefficients:

$$D^{(k)}\left(u_s, s\right) = \lim_{s' \to s} \frac{M^{(k)}\left(u_s, s, \Delta s\right)}{k!\,\left(s' - s\right)}. \quad (2)$$

$D^{(k)}$ can be estimated directly from measured data by an optimization procedure proposed in [1–4], which includes reconstruction of the conditional probability density functions $p\left(u_{s'}|u_s\right)$ via short time propagator [5]. Similarly to previous works, [3, 4, 6–8] we use a linear function for $D^{(1)}$ and a parabolic function for $D^{(2)}$ interpreted in the Itô convention [9]

$$D^{(1)}(u_s, s) = -\alpha u_s, \quad (3)$$

$$D^{(2)}(u_s, s) = \beta + \kappa u_s + \gamma u_s^2 \quad (4)$$

In Fig. 1 the Kramers-Moyal coefficients and the fits for $D^{(1,2)}$ are shown.

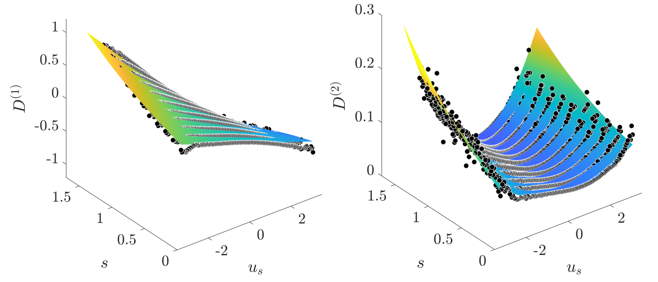


FIG. 1. Kramers-Moyal coefficients $D^{(1,2)}\left(u_s, s\right)$ and surface fits with a linear function for $D^{(1)}\left(u_s, s\right)$ and a parabolic function for $D^{(2)}\left(u_s, s\right)$ (see Eq. (3) - (4)) with respect to scale.

The scale-dependent coefficients $\alpha(s)$, $\beta(s)$, $\kappa(s)$ and $\gamma(s)$ in the fits are estimated using an open-source Matlab package [10] and plotted in Fig. 2. In addition, the constant coefficients of the simplified diffusion model discussed in the primary manuscript with the choice $\alpha = (3 + \mu)/9$, $\beta = 0$, $\kappa = 0$ and $\gamma = \mu/18$, where $\mu = 0.234$ is the standard intermittency parameter [11], are shown.

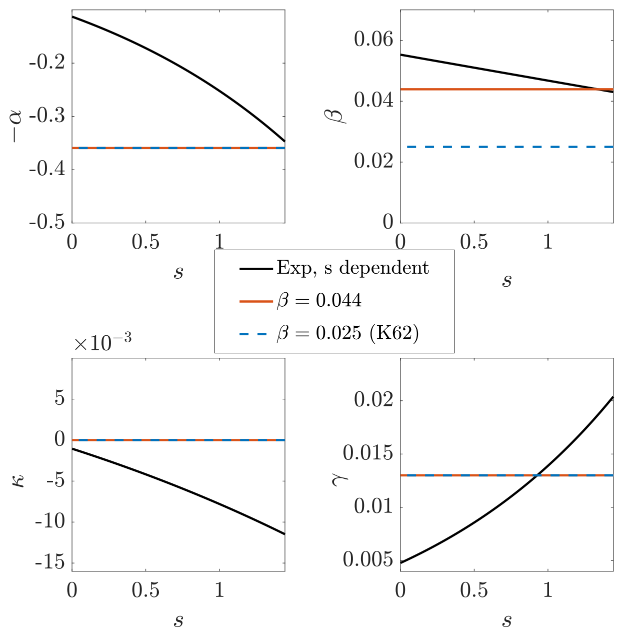


FIG. 2. Scale-dependent coefficients of the Kramers-Moyal coefficients using the surface fits with a linear function for $D^{(1)}\left(u_s, s\right)$ and a parabolic function for $D^{(2)}\left(u_s, s\right)$ (see Eq. (3) - (4)) with respect to scale. Constant coefficients of the simplified diffusion model discussed in the primary manuscript with the choice $\alpha = (3 + \mu)/9$, $\beta = 0$, $\kappa = 0$, $\gamma = \mu/18$ and $\mu = 0.234$.

*Appendix B: Integral fluctuation theorem.*— The next Figure shows the empirical average $\left\langle e^{-\Delta S_{tot}}\right\rangle_N$ as a function of the number $N$ of trajectory sequences $[u(\cdot)]$. The dashed line in the figure corresponds to the integral fluctuation theorem (IFT)

$$\left\langle e^{-\Delta S_{tot}}\right\rangle = \int e^{-\Delta S_{tot}} p\left(\Delta S_{tot}\right) d\Delta S_{tot} = 1, \quad (5)$$

which is a fundamental entropy law for non-equilibrium systems [12, 13]. In Fig. 3 the influence of two values $\beta = 0$ (K62) and $\beta = 0.044$ using a simplified continuous diffusion model discussed in the primary manuscript on the integral fluctuation theorem is presented and compared to the experimental data. We find that K62 theory (log-normal model) is not in agreement with the IFT.

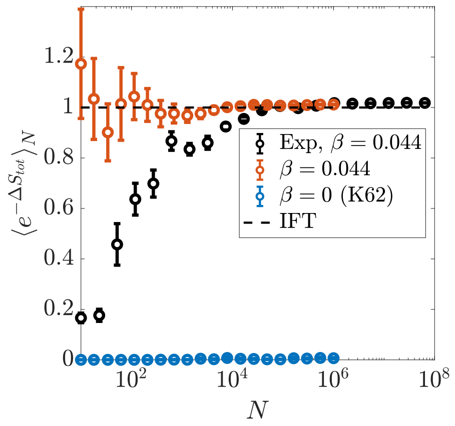


FIG. 3. Empirical average $\langle e^{-\Delta S_{tot}} \rangle_N$ of $\Delta S_{tot}$ as a function of the number $N$ (sample size) of cascade trajectories $[u(\cdot)]$. According to the integral fluctuation theorem, the empirical average has to converge to the horizontal dashed line.

*Appendix C: Cascade trajectories conditioned on* $\Delta S_{med}$.— In Fig. 4, the contours of the PDF of velocity increment conditioned on the entropy exchange $\Delta S_{med}$ are presented as a function of scale for the diffusion model with $\beta = 0$. We find that K62 theory fails to capture the two qualitatively different statistical dynamics conditioned on entropy as shown for the $\beta = 0.044$ model and the experimental data (see primary manuscript Fig. 4). The PDF is concentrated close to the $u_s = 0$ line. There are no distinct lines of maximum probability with a region of very low probability in between. Therefore the K62 instantons conditioned on entropy (black dotted lines in Fig. 4) will always be the trivial path which vanishes everywhere regardless of the imposed value of entropy.

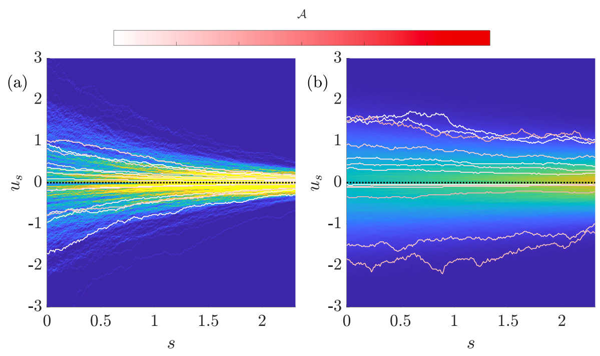


FIG. 4. PDF of velocity increment $u_s$ as a function of scale $s$ (contours), conditioned on (a) $S_{\text{med}} = 50$ and (b) $S_{\text{med}} = -5$ for the numerical data with $\beta = 0$. On top of the PDF are represented randomly chosen cascade trajectories characterized by the same entropy consumption (resp. production), color-coded using the value of their action (increasing from white to red). The black dotted lines represent the instanton trajectories for the model with $\beta = 0$.

*Appendix D: Increment PDFs conditioned on* $\Delta S_{med}$.— In the following the condition on entropy and the influence on the statistics of increments on different scales is examined for the experimental data. In Fig. 5 the PDFs without conditioning on entropy are shown as colored contours. In addition, in Fig. 5 the black contours correspond to the condition on exclusively positive (a) or negative (b) entropy trajectories.

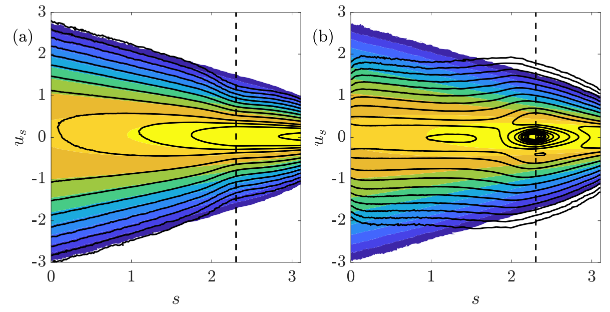


FIG. 5. PDF of velocity increments $u_s$ as a function of scale $s$ for the experimental data without conditioning on entropy are shown as colored contours. In addition, in (a) the condition on exclusively positive entropy trajectories (black contours) and (b) the condition on negative entropy trajectories are plotted. The black vertical dashed line indicates the Taylor length scale.

In Fig. 6 the influence on the histogram (a, c) and the percentage proportion in relation to the full (no condition) data set (b) at the integral scale and (d) Tayor length scale is presented.

In particular, it can be seen that the condition on positive entropy greatly reduces extreme increments at small scales, and nearly all ($\approx 90\%$) of the large increments at small scales (heavy tailed statistics of the small-scale increment PDF) are contained in the negative entropy trajectories. Note, this could be seen as a new approach to the majority of large and intermittent small scale increments.

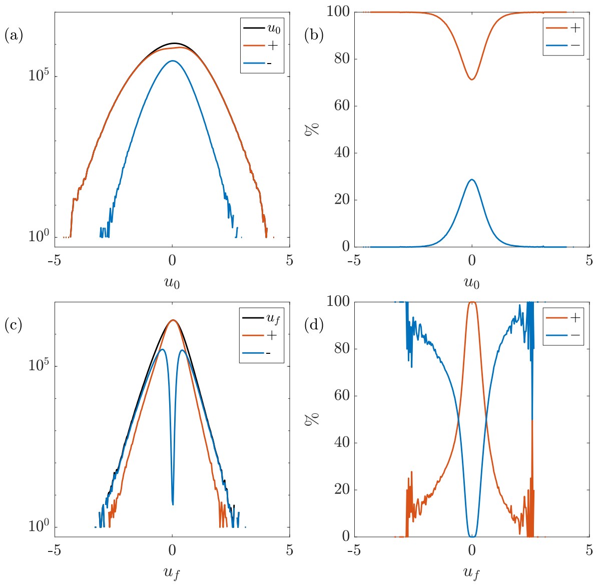


FIG. 6. (a, c): Histogram of velocity increments without conditioning on entropy (black), condition on exclusively positive (red) and negative (blue) entropy trajectories are presented for $u_0$ (a) and $u_f$ (c). (b, d): Percentage proportion in relation to the full (no condition) data set for positive and negative entropy condition.


[1] D. Kleinhans, R. Friedrich, A. Nawroth, and J. Peinke, Phys. Lett. A **346**, 42 (2005).

[2] D. Kleinhans, Phys. Rev. E **85**, 026705 (2012).

[3] A. P. Nawroth, J. Peinke, D. Kleinhans, and R. Friedrich, Phys. Rev. E **76**, 056102 (2007).

[4] N. Reinke, A. Fuchs, D. Nickelsen, and J. Peinke, J. Fluid Mech. **848**, 117 (2018).

[5] H. Risken, *The Fokker-Planck Equation*, 2nd ed. (Springer, 1989).

[6] C. Renner, J. Peinke, and R. Friedrich, J. Fluid Mech. **433**, 383 (2001).

[7] C. Renner, J. Peinke, R. Friedrich, O. Chanal, and B. Chabaud, Phys. Rev. Lett. **89**, 124502 (2002).

[8] A. Fuchs, S. M. D. Queirós, P. G. Lind, A. Girard, F. Bouchet, M. Wächter, and J. Peinke, Phys. Rev. Fluids **5**, 034602 (2020).

[9] C. W. Gardiner, *Handbook of Stochastic Methods for physics, chemistry, and the natural sciences*, 4th ed. (Springer, Berlin, 2009).

[10] A. Fuchs, S. Kharche, M. Waechter, and J. Peinke, "An open source matlab package for solving fokker-plank equation and validation of integral fluctuation theorem," .

[11] R. Friedrich and J. Peinke, Phys. Rev. Lett. **78**, 863 (1997).

[12] U. Seifert, Phys. Rev. Lett. **95**, 040602 (2005).

[13] U. Seifert, Rep. Prog. Phys. **75**, 126001 (2012).
